# Supplementary material for: Spatial Coherence Properties of Organic Molecules Coupled to Plasmonic Surface Lattice Resonances in the Weak and Strong Coupling Regimes
Source: arXiv:1404.4160 source file (2014-04-16)
Supplement: Supplementary file 1 [file Supplemental_Material.pdf]

# Spatial Coherence Properties of Organic Molecules Coupled to Plasmonic Surface Lattice Resonances in the Weak and Strong Coupling Regimes

Supplemental Material

L. Shi, T. K. Hakala, H. T. Rekola, J. -P. Martikainen, R. J. Moerland, and P. Törmä

COMP Centre of Excellence, Department of Applied Physics, Aalto University, FI-00076 Aalto, Finland

## The fabrication of the nanoparticle arrays and the absorbance of the bare DiD dye film

In Fig. 1 are shown the scanning electron micrographs (SEM) of a typical periodic and a random nanoparticle sample. The nanoparticle orientation, size and number were equal for both samples. The samples were fabricated with electron beam lithography and metal evaporation (Ti 2 nm / Ag 30 nm) on a borosilicate substrate. Several 40µm x 40µm arrays were fabricated with different particle lengths d and periodicities p, see Fig. 1(a) of the manuscript. The $d_y$ = 50 nm for all the particles while $d_x$ was varied from 133 nm to 400 nm for different arrays. Also, $p_y$ was kept constant (200 nm) while $p_x$ was systematically varied between 380-500 nm. The DiD molecules were mixed with poly(methyl methacrylate)–anisole solution and the resulting mixture was then spun cast onto the samples resulting to DiD concentrations from 20 mM to 800 mM in the film. Prior to the measurements, the sample was covered with index matching oil and another borosilicate slide to provide a symmetric refractive index environment.

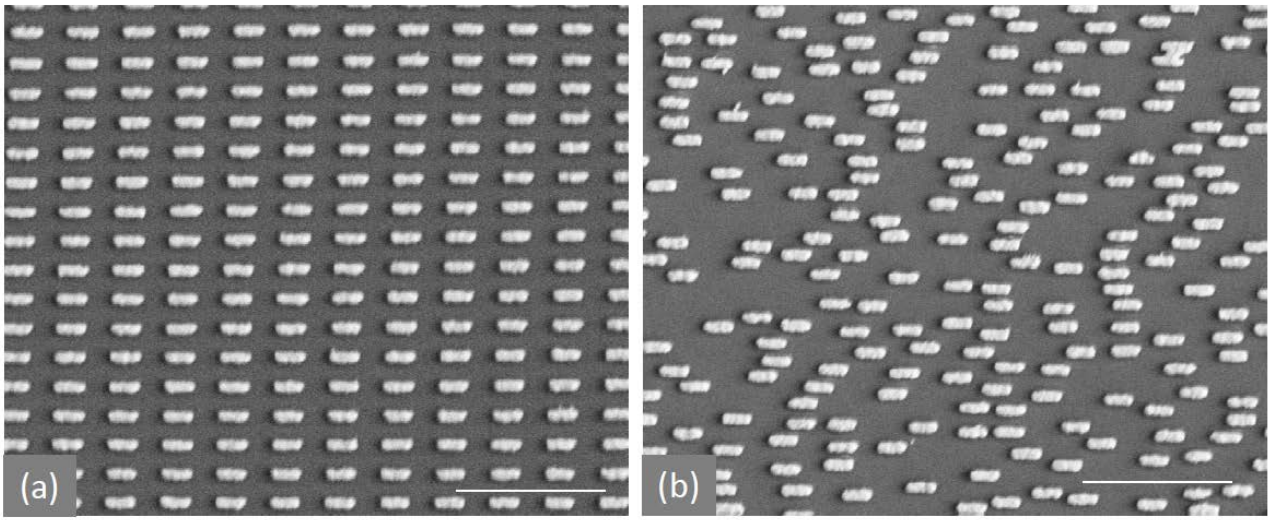


Fig. 1. SEM of a typical nanoparticle array (a) and a random sample (b). The scale bars are 1 $\mu$m.

## The effect of increasing filling fraction: Bright and dark modes

The coupling of <+1, 0> and <-1, 0> diffractive orders in periodic structures leads to formation of a band gap. By changing the filling fraction either of the modes can be made dipole active. This can be seen in Fig. 2, where the extinction data is plotted for 6 different arrays with increasing filling fraction $d_x$ / $p_x$. No DiD film was present in this case. The periodicity $p_x$ = 460 nm, $p_y$ = 200 nm and $d_y$ = 50 nm for all the arrays, while the $d_x$ was varied from 161 nm to 368 nm.

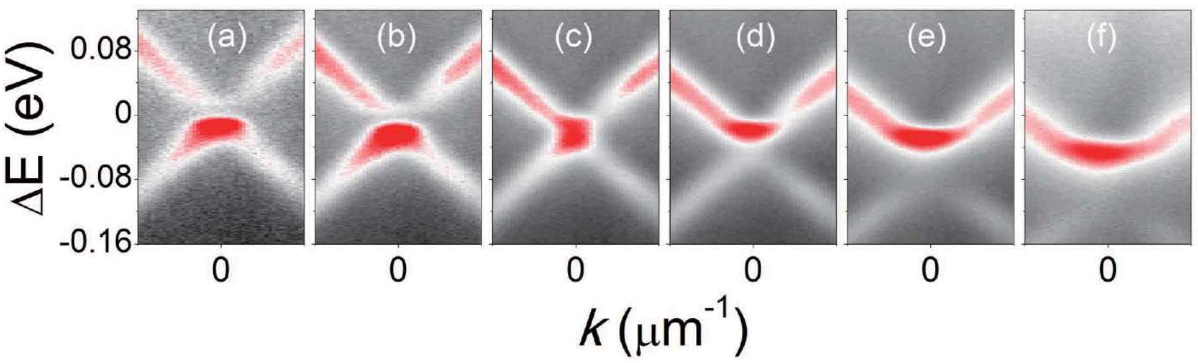


Fig. 2. The effect of increasing filling fraction $d_x / p_x$ (see manuscript Fig. 1(a)) from 35 % to 80 % (in steps of 9%). The extinction maximum shifts from the lower energy branch to the higher energy one. The red (black) color corresponds to the highest (lowest) extinction.

**DiD dye absorption**

In Fig. 3 are shown the measured absorption curves from DiD films with various concentrations. Also shown are the two Gaussians and their sum fitted to the absorption curves in order to find the center energies for DiD film absorption at each concentration. These energies were then used as uncoupled DiD absorption energies in the coupled oscillator model.

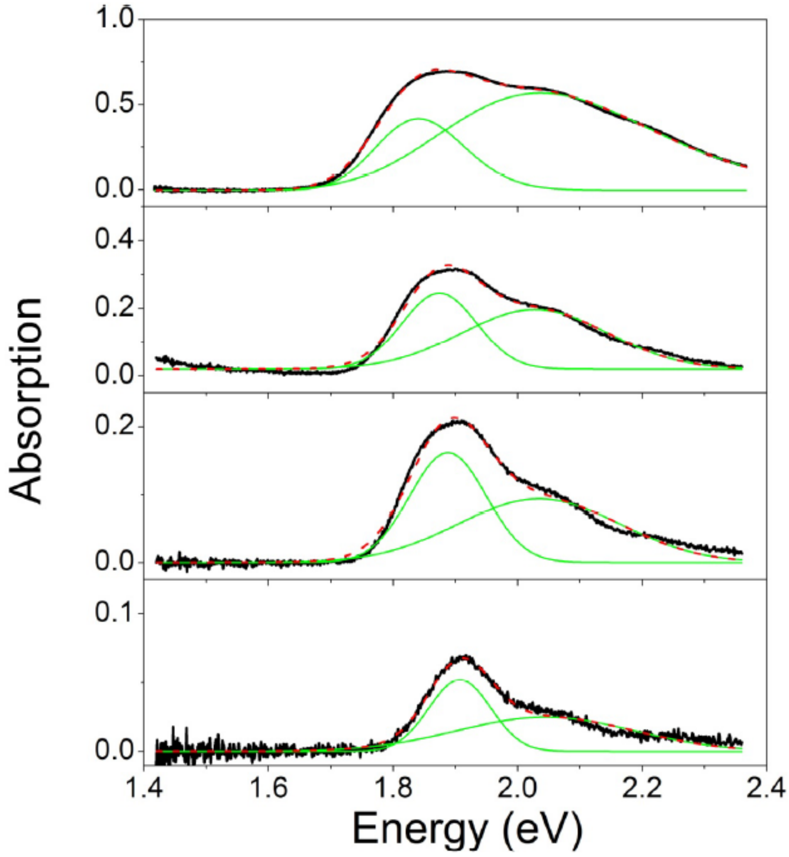


Fig. 3. The measured absorption curves (from top to bottom) for the DiD films with concentrations 800 mM, 400 mM, 200 mM, and 50 mM, respectively. Also shown are the two fitted Gaussians (green solid lines) and their sum (dashed red line).

**Obtaining the *E*, $\gamma$ and $\Delta k$ from the measured extinction curves**

From the measured dispersion data, the mode energy *E* (the peak of the red solid curve, see Fig. 4) and the width $\gamma$ (FWHM of the red solid curve) were obtained for each *k*. The mode energies were then plotted as yellow symbols in Fig. 2 and 3 in the manuscript. As in [1], $\gamma$ was then used to define the uncertainty in the parallel wavevector $\Delta k$, see Fig. 4.

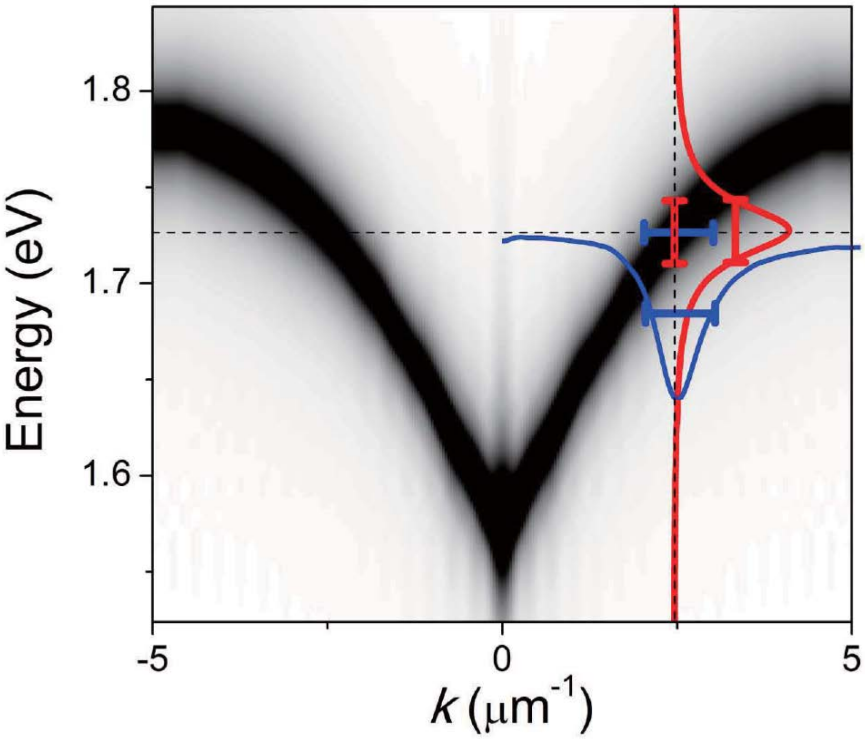


Fig. 4. The mode energy *E(k)* (the peak of the red solid curve) and the width $\gamma$ (FWHM of the red solid curve) were obtained from the measured extinction data for each *k*.

**Obtaining the relevant parameters for the coupled oscillator model**

The parameters for the coupled oscillator model (See Eq. (1) of the manuscript) were obtained as follows. The energy $E_{SLR}(k)$ and the width $\gamma_{SLR}$ of the uncoupled SLR mode were obtained from the measurements without the DiD film for each array, and the uncoupled DiD absorption energies $E_{DiD}$ were obtained from the transmission measurements of the bare DiD film without any nanoparticles, see Fig. 3. For fitting, the SLR-DiD coupling strength $\Omega$ and the width of the DiD absorption $\gamma_{DiD}$ were used as free parameters. Obtained by diagonalization of the matrix in Eq. 1 of the manuscript, the resulting hybrid mode eigenenergies were plotted as red symbols in Fig. 2 (c-e), (h-j) and (m-o) in the manuscript. Note that for 20 mM and 50 mM DiD concentration, the eigenenergies were essentially the same as in the absence of the dye, so the fitting resulted to negligible coupling strength (see Figs. 7-9 in the Supplemental Information and Fig. 2(p) in the manuscript). For the same reason, the obtained relative SLR-exciton weights are plotted only for the three largest DiD concentrations (200 mM, 400 mM and 800 mM) in Fig.2(q-s) in the manuscript.

**Comparison between microscopic theory and experimental results**

To estimate the size of the splitting in dispersions from first principles, we employ the light-matter strong coupling theory (see e.g. [1, 2]). Here, we directly quote the results given in reference [1], using corresponding microscopic quantities in our system. Accounting for a random orientation of the dye molecules in the system, the final coupling strength ***Ω*** can be calculated as $\Omega = \sqrt{\Omega_0^2 - (\frac{\gamma_{SLR}^2 + \gamma_{DiD}^2}{2})} = \sqrt{\frac{d^2 E_{DiD}^2}{4\varepsilon_0 \varepsilon_b E_{SLR}(0)} \times \frac{N}{V_{SLR}} - (\frac{\gamma_{SLR}^2 + \gamma_{DiD}^2}{2})}$ , where *d* is the intrinsic transition dipole moment of a single DiD molecule, $\boldsymbol{\varepsilon_b}$ is the relative permittivity of the background material, *N* is the number of the molecules enclosed by the optical field of the SLR and $V_{SLR}$ is the mode volume of the SLR.

In Fig. 5, we compare our experimental results with the microscopic model. We would like to emphasize that, to the best our knowledge, this is the first (or at least one of the first) report(s) where a detailed comparison between experimentally observed splittings and microscopic predictions is made. The experimental results are the same as the data shown in the manuscript. In Fig. 5(a), the results from the microscopic model are calculated by directly using the values of the intrinsic dipole moment and the concentration of the DiD dye from the literature and our experiments without any further fitting parameters. The intrinsic dipole moment of a single DiD molecule is reported to be approximately $5*10^{-29}$ Cm [3]. The $E_{DiD}$, $E_{SLR}$, $\gamma_{DiD}$ and $\gamma_{SLR}$ are obtained from the experimental results of the uncoupled SLR dispersion and DiD absorption, shown in Fig. 2(a, f and k) of the manuscript and Fig. 2 in the Supplemental Information. The $\boldsymbol{\varepsilon_b}$ = 2.3. The $\frac{N}{V_{SLR}}$ equals the nominal concentration of the DiD dye in the polymer film. While the results from the microscopic model have the same linear dependence on the concentration as the experimental results, the obtained mode splitting is approximately 3 times higher. The discrepancy likely stems from various reasons, namely 1) the exact value of the dipole moment of the DiD molecule in our system may well be different from the value reported in [3], 2) in the experiments, only the top surface of the lattice structure is coated by the dye molecules, effectively reducing the magnitude of $\frac{N}{V_{SLR}}$ term, 3) the possible aggregation of the DiD molecules, leading to effectively lower concentration, is neglected in our model.

Next, we will, one by one, analyze the influences of the aforementioned aspects to the final coupling strength. First, if we leave the intrinsic dipole moment to be a free parameter, and using the experimental data to fit the intrinsic dipole moment, we obtain results are shown in Fig. 5(b). The obtained intrinsic dipole moment of a single DiD dye is $1.58*10^{-29}$ Cm, which is in the same order of the reported value [3] but approximately 3 times less. Second, approximately one half of the field of the SLR mode resides in the glass substrate where no DiD is present. Thus the value of $\frac{N}{V_{SLR}}$ could be naively estimated to be half of the nominal concentration of the DiD dye in the polymer film. Taking into account this fact, and still using the reported DiD dye intrinsic dipole moment ($5*10^{-29}$ Cm), we then obtain a coupling strength shown in Fig. 5(c). Obviously, the value is approaching the experimental results. Third, it is reasonable to assume that some of the DiD dye molecules aggregate in the polymer film, which results to the reduction of the effective DiD concentration. Despite the complexity of our system, it is interesting to find that there still exists a reasonable agreement between the results calculated from the first principles and the experimental data.

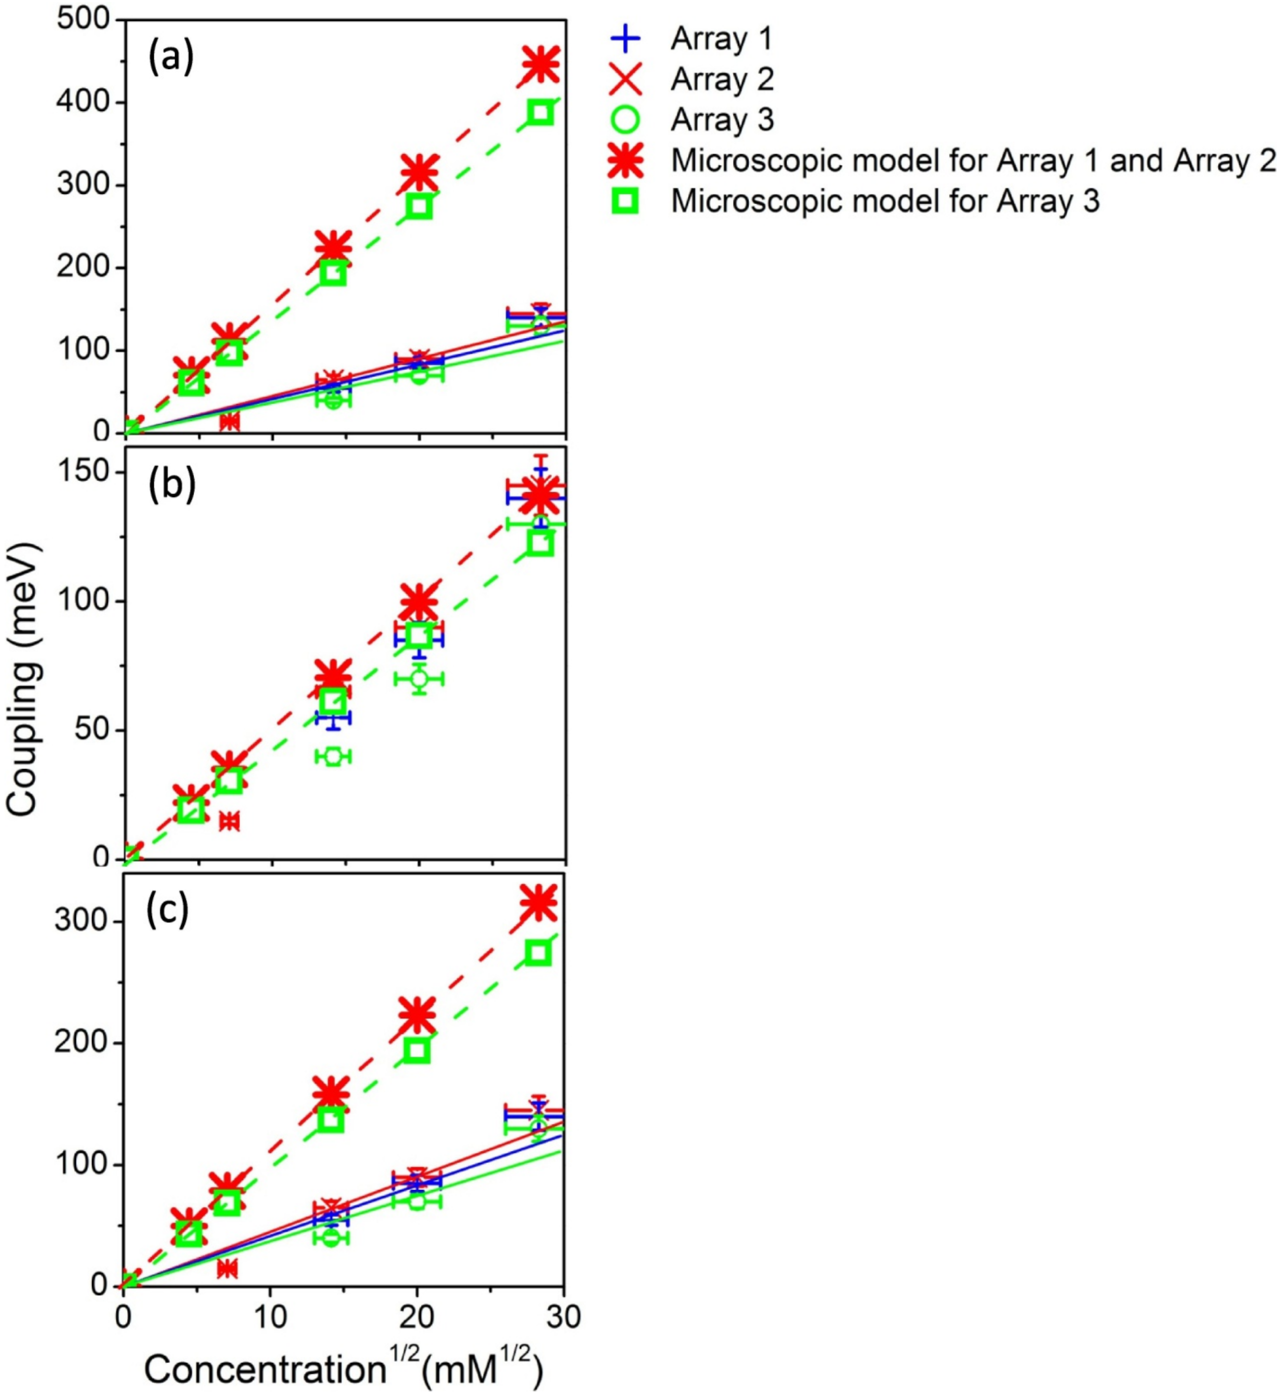


Fig. 5. The coupling strength obtained from microscopic model and experimental results. The symbols and their meaning are represented inside the figure. The experimental data shown here is the same as the Fig. 2(p) of the manuscript. The microscopic model results shown in (a and c) correspond to the case of $5*10^{-29}$ Cm intrinsic transition dipole moment of single DiD molecule, while (b) corresponds to the case of $1.58*10^{-29}$ Cm intrinsic transition dipole moment of single DiD molecule. In (a and b), the $\frac{N}{V_{SLR}}$ equal to the concentration of the DiD dye in the polymer film, and in (c), the $\frac{N}{V_{SLR}}$ equal to the half of the concentration of the DiD dye in the polymer film.

**Generating the spatial coherence image from the coupled oscillator model**

To generate the diffraction pattern from the coupled oscillator model (see Fig. 4(b) in the manuscript), the following procedure was applied: For every $k$, the eigenenergies $E(k)$ and the widths $\gamma$ of the strongly coupled mode were given by the real and imaginary parts of the diagonalized matrix (Eq. (1)), respectively. Then, for each $k$, we assumed a Lorentzian lineshape $f(E)$, whose center and width were given by $E(k)$ and $\gamma$, respectively. These Lorentzians were used to construct a 2-D contour map $f(E, k)$, similar to experimentally obtained dispersion. This dispersion was then used to provide the energy and wavelength specific information of the mode radiating through the double slit.

By taking an inverse Fourier transform of the obtained dispersion $f(E, k)$, the real-space intensity distribution $f'(E, x)$ of the mode at the position of the double slit was obtained for each $E$. The double slit transmission $\Phi(x)$ was assumed to be 1 at the slit openings and 0 elsewhere. The transmitted field $\Phi(x) \times f'(E, x)$ was then Fourier transformed to obtain the spatial coherence image.

**Spatial coherence images with various double slit configurations**

In Fig. 6 are shown the spatial coherence images in various slit configurations for the periodic structure (a, c and e) and for the random structure (b, d and f). Figs. 6(a) and (b) correspond to the experiments without double slit, (c) and (d) with double slit and (e) and (f) with one of the slits blocked so that only one slit is transmitting light. The concentration of the DiD is 800 mM. Note that in the absence of the double slit (Figs. 6(a) and (b)), the periodic structure displays a $k$-dependent dispersion, while the random structure shows two $k$-independent transmission minima at 1.8 eV and 2.25 eV, corresponding to DiD main absorption and single particle surface plasmon resonance, respectively. Note also an additional, very faint transmission minimum at around 2.05 eV in Fig. 6(b) that corresponds to the DiD absoption shoulder, see Fig. 3. By placing a double slit to the image plane of the sample, a distinct interference pattern is obtained from the periodic sample due to delocalized mode (Fig. 6 (c)), while the random sample maintains the two $k$-vector independent transmission minima. In the case of only single slit (Fig. 6(e)), the interference pattern from the periodic array disappears almost entirely. The mode delocalization is in this case limited by the effective slit width (3.5 $\mu$m), which effectively increases the $\Delta k$ and reduces the interference effects. In contrast, the transmission of the sample with randomly distributed nanoparticles remains the same even in the presence of the single slit since the mode coherence length is smaller than the slit width, see Fig. 6(f).

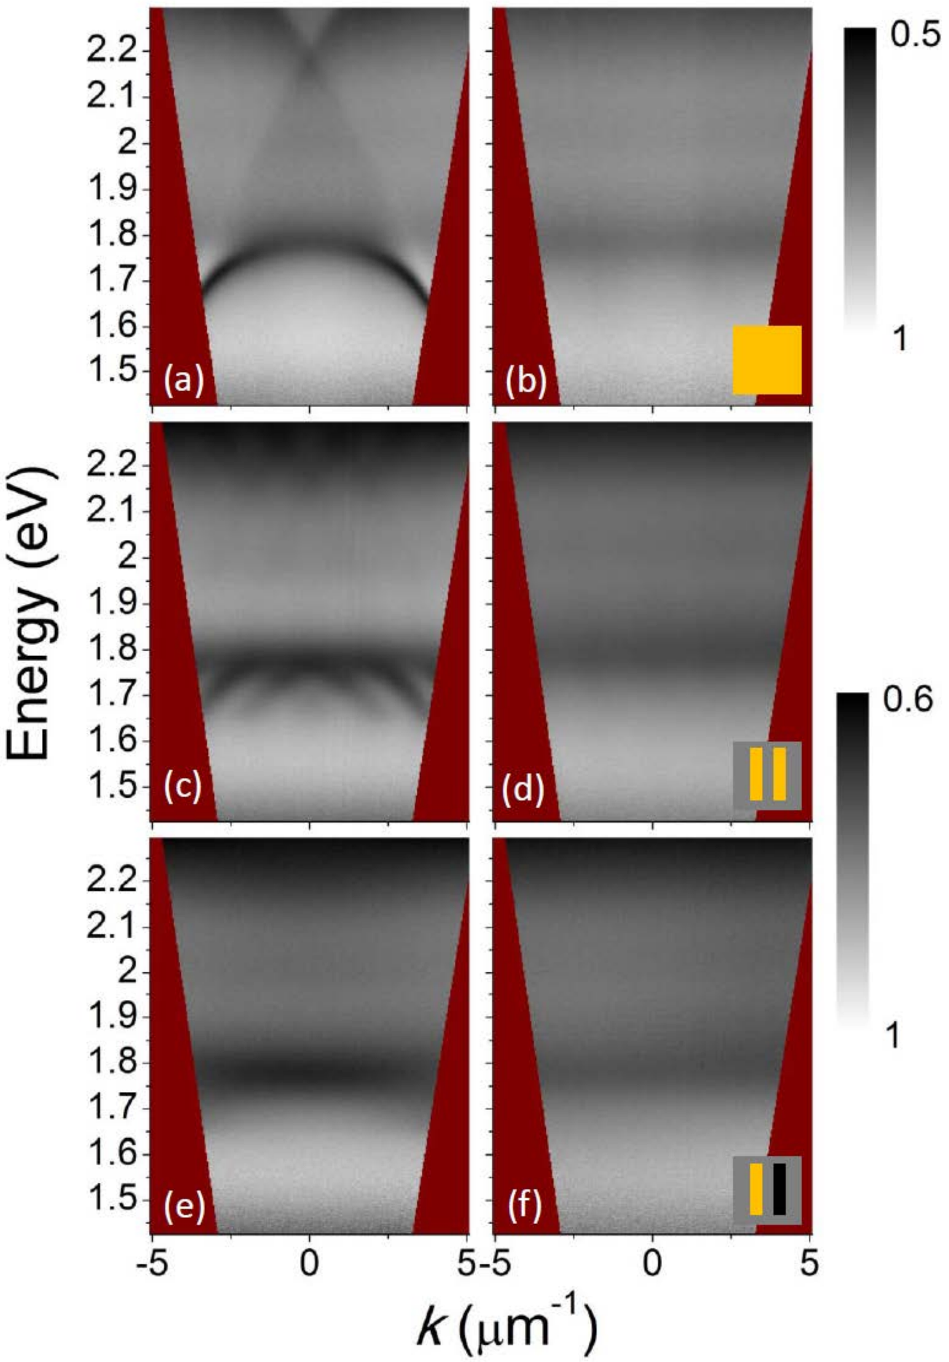


Fig. 6. The transmission intensities as functions of the parallel wavevector and the energy for the cases of the periodic structure (a, c and e) and the random structure (b, d and f). (a, b), (c, d) and (e, f) correspond to the experiments without double slit (shown inset of the (b)), with double slit (shown inset of the (d)) and with single slit (shown inset of the (f)) respectively. The concentration of the DiD is 800 mM. The periodic sample has dimensions $d_x$ = 201 nm, $d_y$ = 50 nm, $p_x$ = 380 nm, $p_y$ = 200 nm. Similar behavior can be seen for the array 3 in the manuscript which has approximately similar nominal dimensions (compare Fig. 6 (a) above to Fig. 2 (o) of the manuscript). In this case, the DiD exciton couples strongly with the *lower* energy branch of the SLR, while still maintaining the significant spatial coherence length as evidenced by the distinct interference pattern (see Fig. 6 (c) above).

**The measured raw extinction data for various array dimensions and DiD concentrations**

While the data in the manuscript is based on 3 different arrays for the sake of simplicity, altogether 24 different arrays with different dimensions were measured. We used 6 different molecular concentrations, 0 mM, 20 mM, 50 mM, 200 mM, 400 mM and 800 mM. The measured extinction data is shown in Figs. 7-12. Below are shown the dimensions for each array. Particle dimensions are in the form ($d_x$ x $d_y$) and period dimensions in the form ($p_x$ x $p_y$), see Fig. 1(a) in the manuscript. Note that the dimensions were chosen such that each *column* in Figs. 7-12 has the same filling fraction $d_x / p_x$ while each *row* has the same periodicity $p_x$. The data is organized in such a way that a certain array always corresponds to the same letter (a, b, c, etc.). The white (black) color corresponds to the highest (lowest) extinction in all figures.

(a) 175.0x50.0 $nm^2$ particles with 500.0x200.0 $nm^2$ period

(b) 220.0x50.0 $nm^2$ particles with 500.0x200.0 $nm^2$ period

(c) 265.0x50.0 $nm^2$ particles with 500.0x200.0 $nm^2$ period

(d) 310.0x50.0 $nm^2$ particles with 500.0x200.0 $nm^2$ period

(e) 355.0x50.0 $nm^2$ particles with 500.0x200.0 $nm^2$ period

(f) 400.0x50.0 $nm^2$ particles with 500.0x200.0 $nm^2$ period

(g) 161.0x50.0 $nm^2$ particles with 460.0x200.0 $nm^2$ period

(h) 202.0x50.0 $nm^2$ particles with 460.0x200.0 $nm^2$ period

(i) 244.0x50.0 $nm^2$ particles with 460.0x200.0 $nm^2$ period

(j) 285.0x50.0 $nm^2$ particles with 460.0x200.0 $nm^2$ period

(k) 327.0x50.0 $nm^2$ particles with 460.0x200.0 $nm^2$ period

(l) 368.0x50.0 $nm^2$ particles with 460.0x200.0 $nm^2$ period

(m) 147.0x50.0 $nm^2$ particles with 420.0x200.0 $nm^2$ period

(n) 185.0x50.0 $nm^2$ particles with 420.0x200.0 $nm^2$ period

(o) 223.0x50.0 $nm^2$ particles with 420.0x200.0 $nm^2$ period

(p) 260.0x50.0 $nm^2$ particles with 420.0x200.0 $nm^2$ period

(q) 298.0x50.0 $nm^2$ particles with 420.0x200.0 $nm^2$ period

(r) 336.0x50.0 $nm^2$ particles with 420.0x200.0 $nm^2$ period

(s) 133.0x50.0 $nm^2$ particles with 380.0x200.0 $nm^2$ period

(t) 167.0x50.0 $nm^2$ particles with 380.0x200.0 $nm^2$ period

(u) 201.0x50.0 $nm^2$ particles with 380.0x200.0 $nm^2$ period

(v) 236.0x50.0 $nm^2$ particles with 380.0x200.0 $nm^2$ period

(w) 270.0x50.0 $nm^2$ particles with 380.0x200.0 $nm^2$ period

(x) 304.0x50.0 $nm^2$ particles with 380.0x200.0 $nm^2$ period

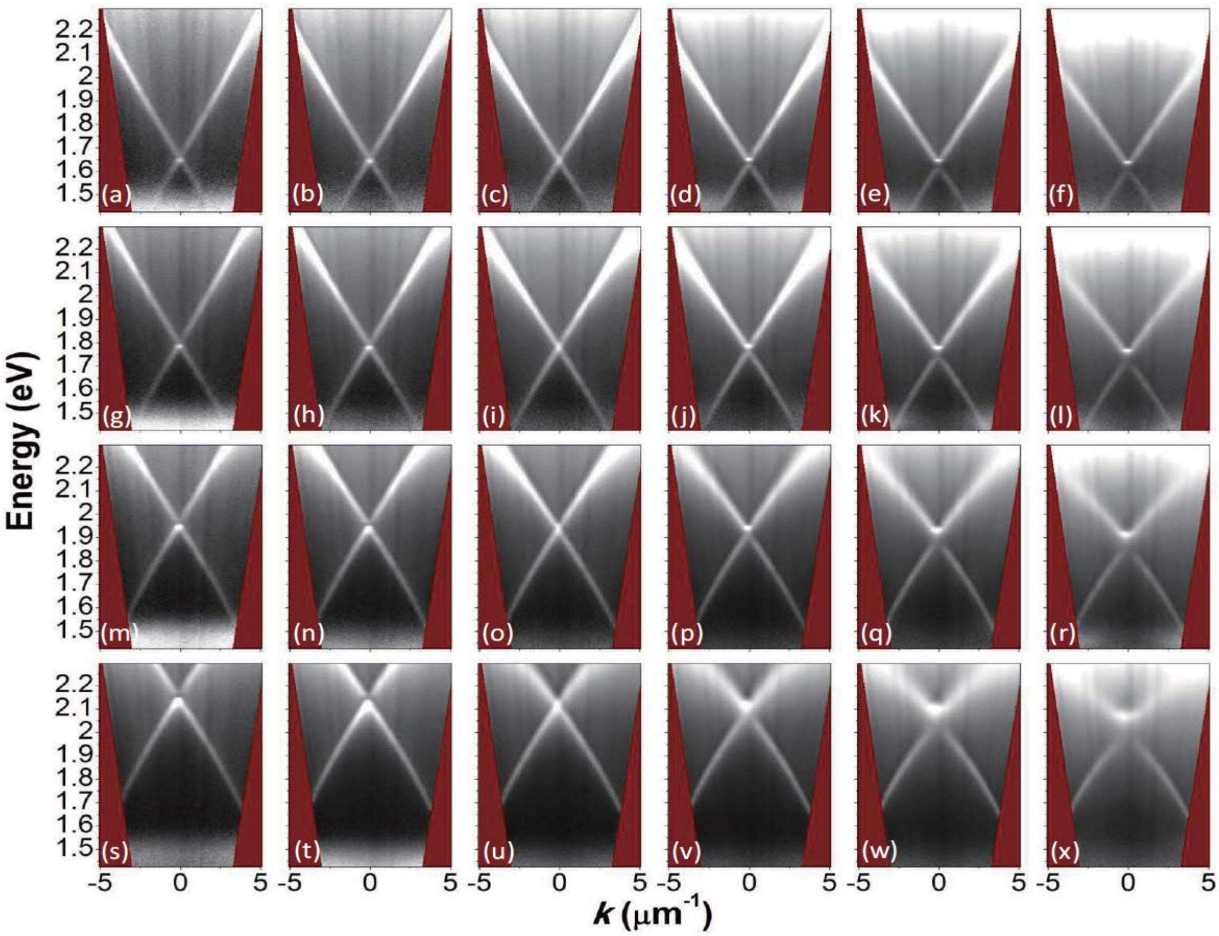


Fig. 7. The recorded raw extinction data for the arrays without any DiD film (0 mM case). The white (black) color corresponds to the highest (lowest) extinction.

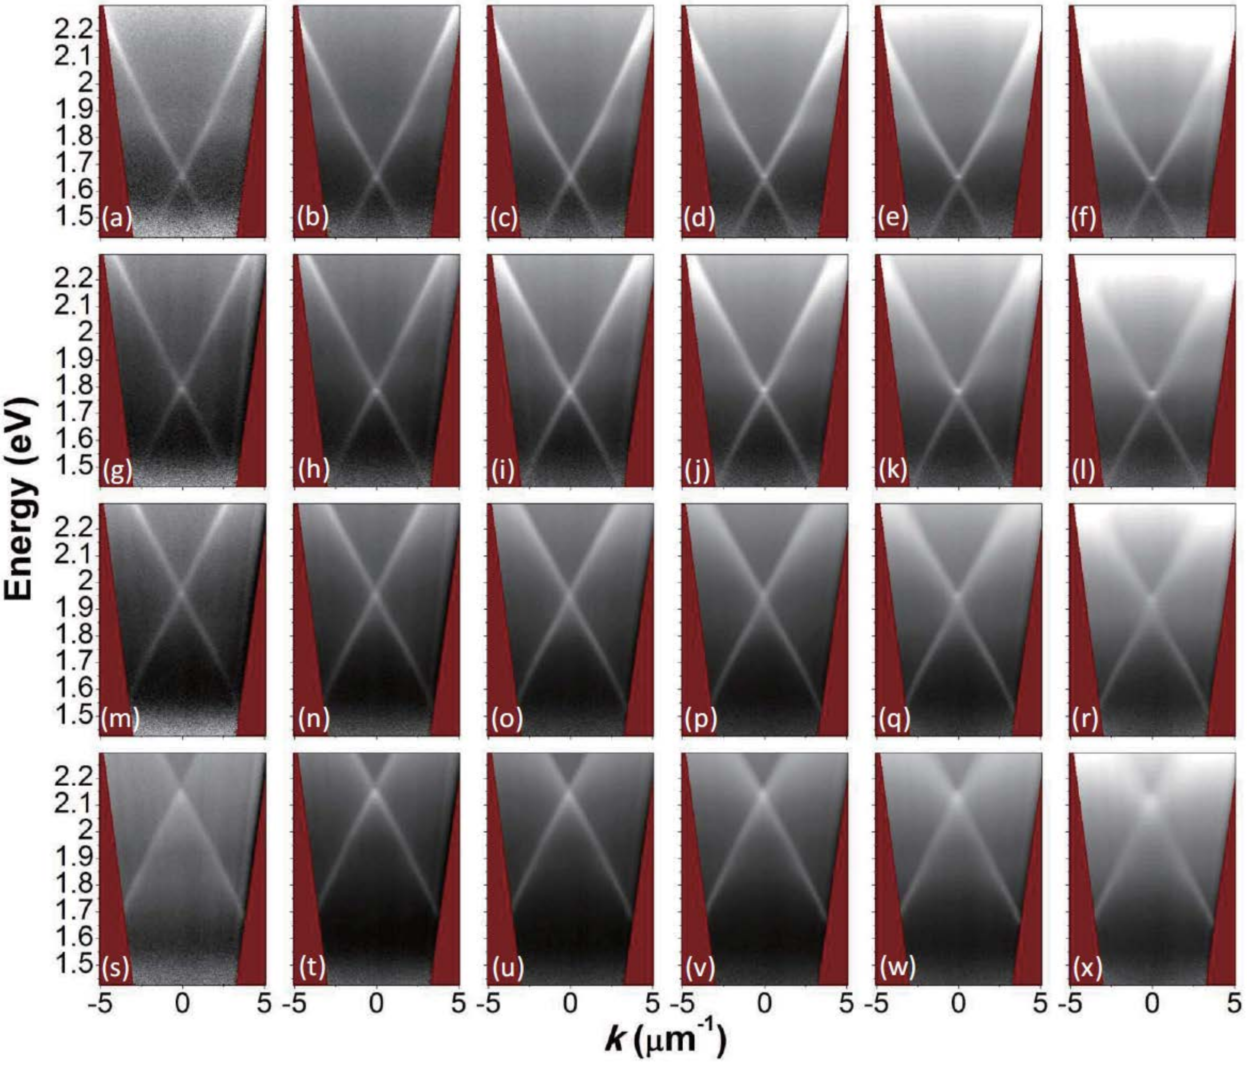


Fig. 8. The recorded raw extinction data for the arrays with 20 mM DiD concentration. The white (black) color corresponds to the highest (lowest) extinction.

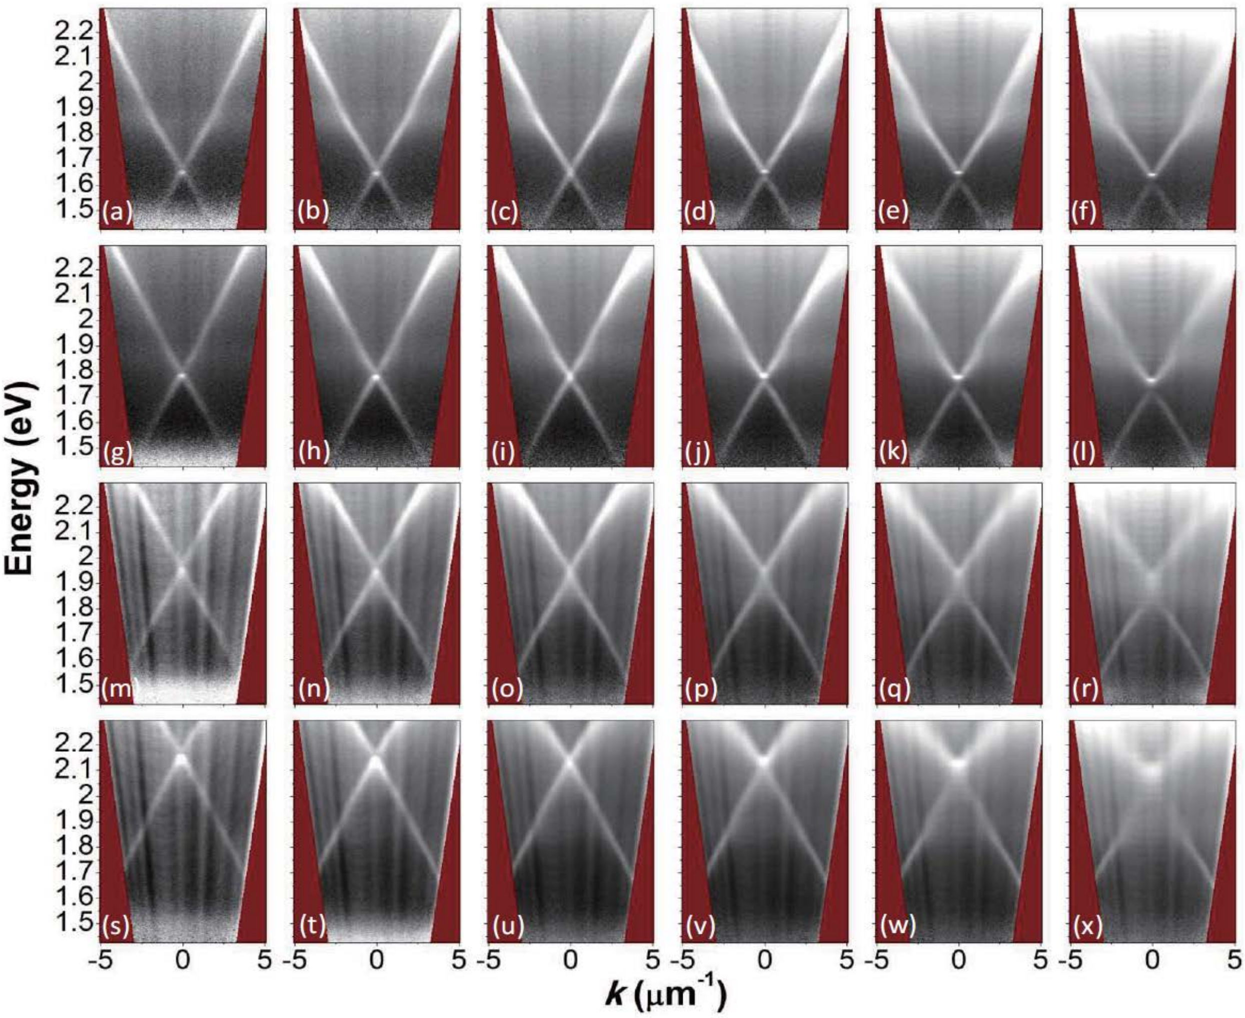


Fig. 9. The recorded raw extinction data for the arrays with 50 mM DiD concentration. The white (black) color corresponds to the highest (lowest) extinction.

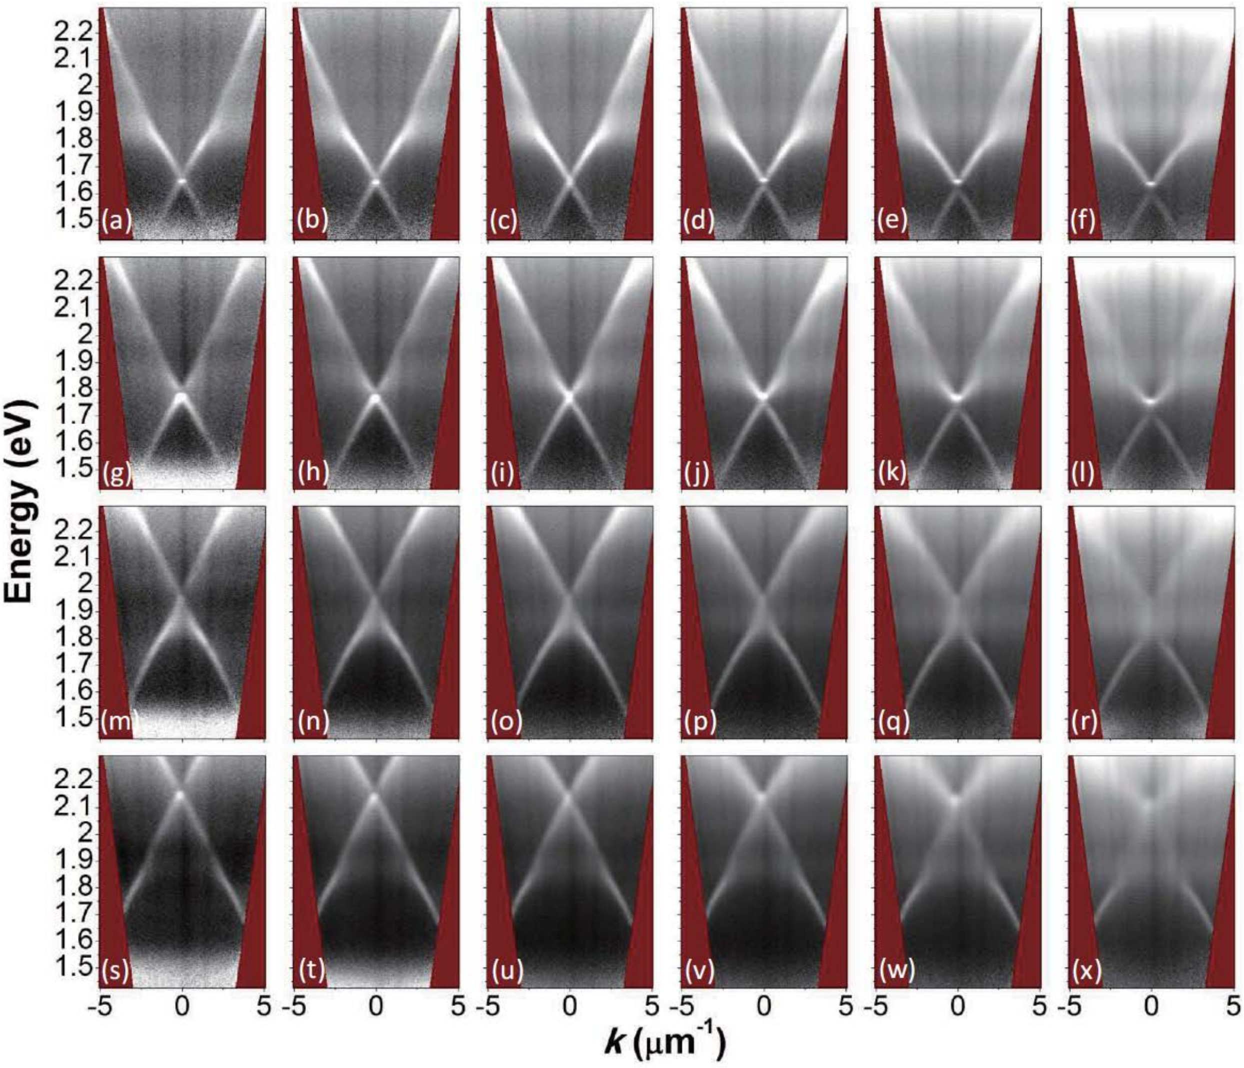


Fig. 10. The recorded raw extinction data for the arrays with 200 mM DiD concentration. The white (black) color corresponds to the highest (lowest) extinction.

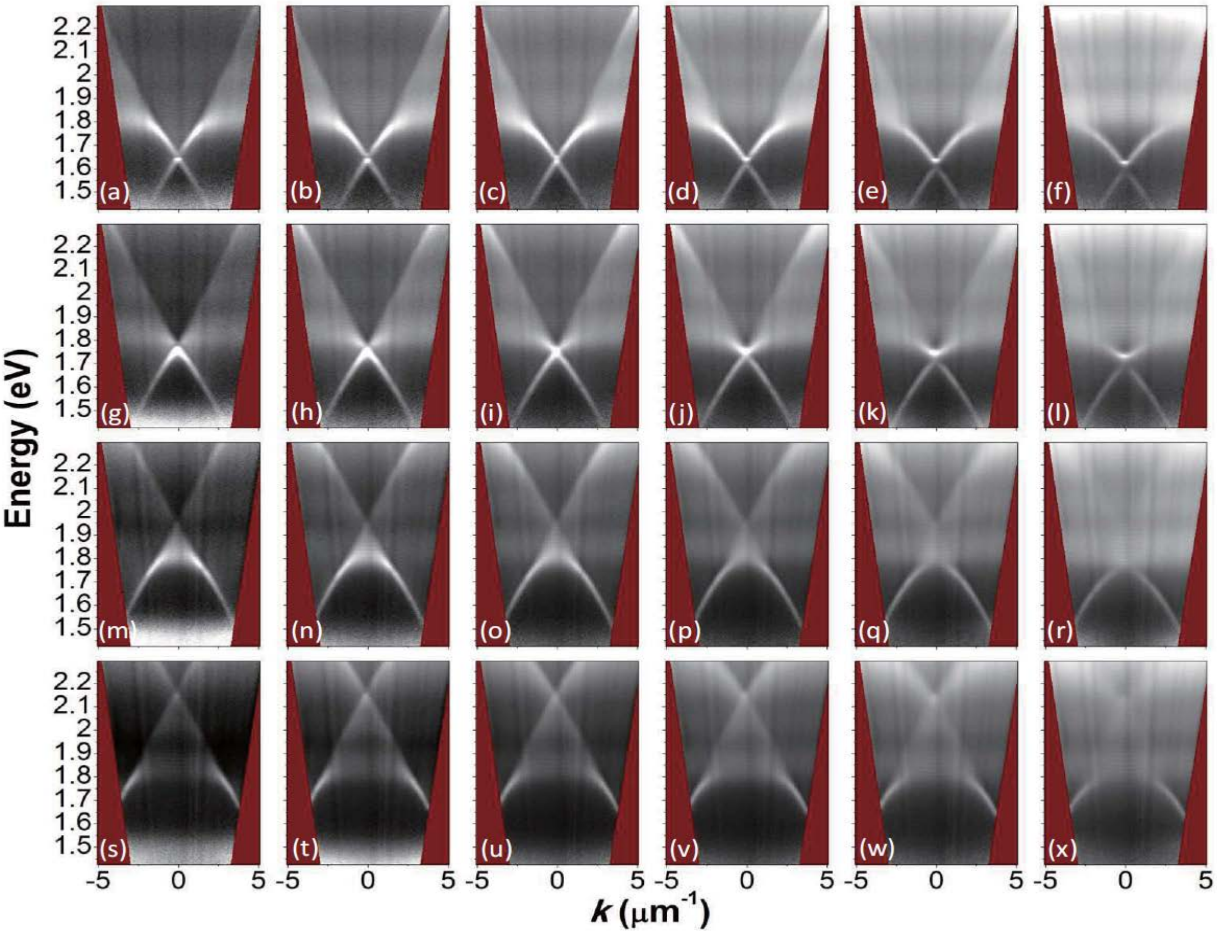


Fig. 11. The recorded raw extinction data for the arrays with 400 mM DiD concentration. The white (black) color corresponds to the highest (lowest) extinction.

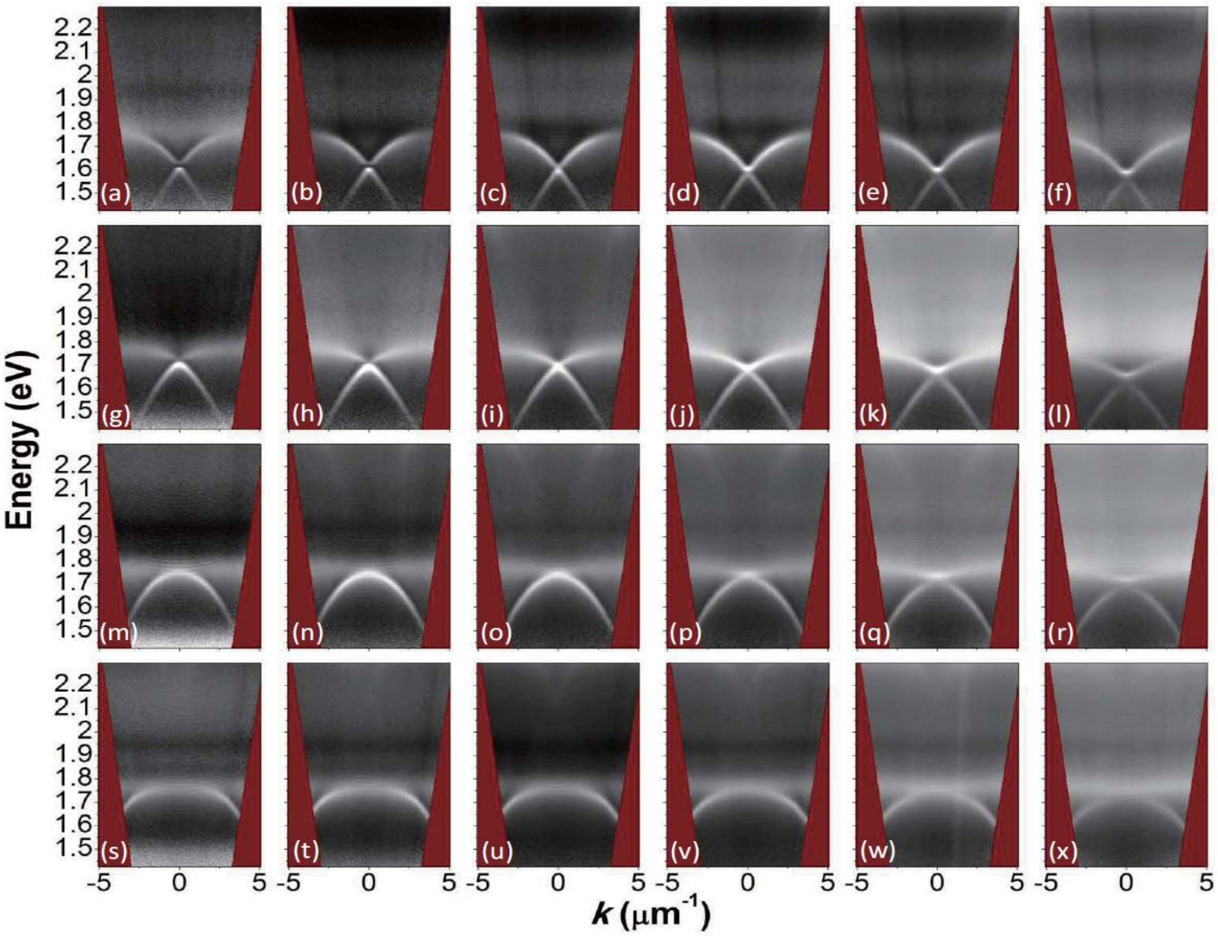


Fig. 12. The recorded raw extinction data for the arrays with 800 mM DiD concentration. The white (black) color corresponds to the highest (lowest) extinction.

**The connection between the measured dispersion curves and the observed interference patterns**

As pointed out in the manuscript, there exists an intimate connection between the measured dispersion curves and the observed spatial coherence images. In particular, one of the destructive interference fringes in the spatial coherence images always overlaps with the extinction maxima of the dispersion (yellow symbols), see manuscript Figs. 3 (a-d). This is because the spatially coherent light source (the sample) is radiating through a double slit. The slit effectively creates replicas of the original dispersion with equal spacing in k. The dark areas in the spatial coherence images correspond to the overlap region of the diffracted orders. However, in a strongly coupled system (for example with 400 mM and 800 mM DiD concentrations) the slope of the dispersion is reduced at large k-vector values, and the energy difference between the areas is reduced, making it harder to distinguish between the different orders. Figure 13 (a) illustrates this.

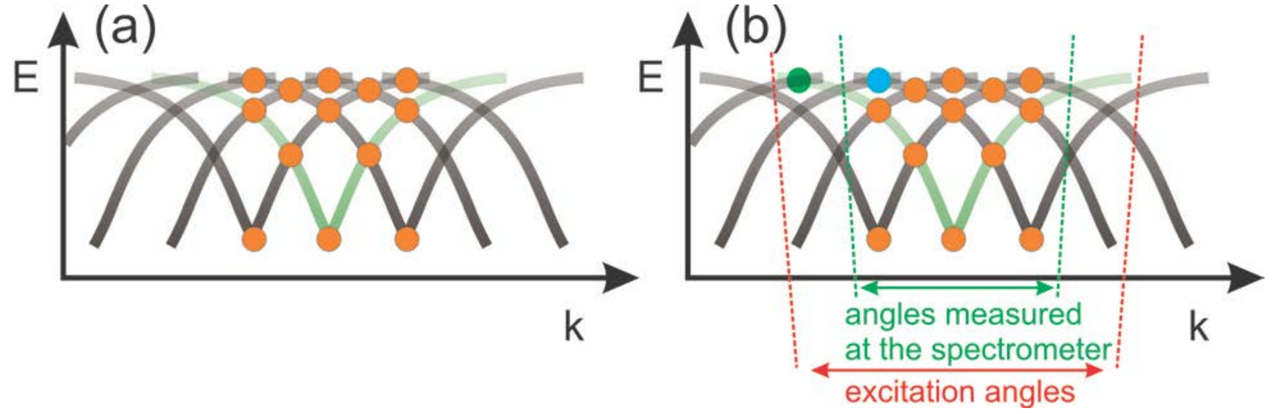


Fig. 13. (a) A schematic representation of the connection between the dispersion and the interference pattern. The double slit produces replicas (depicted as grey solid lines) of the original dispersion (depicted as green solid lines). The dark areas in the spatial coherence images correspond to the overlap region of the diffracted orders (here depicted as orange circles). In the strongly coupled system (400 mM and 800 mM concentrations) the slope of the dispersion is reduced at large k-vector values, and the energy difference between these areas is decreased, thus creating a complex interference pattern. (b) Some information is lost when generating an interference image from the measured dispersion due to the limited size of the CCD detector in the spectrometer: the angle distribution in the excitation light incident on the sample (depicted as red dashed lines) is larger than the range of angles that the spectrometer is able to measure due to the limited size of the CCD detector (depicted as green dashed lines). Thus some part of the incident light (such as the green circle), is still contributing to the measured interference image (the blue circle in the image) because it is effectively folded on a smaller momentum at the double slit plane, but it cannot be numerically reproduced from the measured dispersion data.

The effect creates a complex pattern in the interference image. To provide more information about the connection between the dispersion and the interference pattern, we numerically reproduced the interference images by (1) taking a fast Fourier transform (FFT) of the measured dispersion to obtain the real space distribution of the field after the sample, (2) used a spatial filter corresponding to the double slit (transmission = 1 at the spatial location corresponding to the slit openings and 0 elsewhere), and (3) performed an inverse FFT to the field transmitted by the double slit. In Fig. 14, the dispersion, the numerically generated spatial coherence image from the measured dispersion image, and the experimentally obtained spatial coherence images are shown for both 400 mM and 800 mM concentrations. The areas of destructive interference follow closely the extinction maxima of the dispersion (the yellow line). The numerically obtained interference patterns in Figs. 14 (b), (e) show slightly higher interference fringe contrast at high energies (1.75-1.8 eV) than the measured ones in Figs. 14 (c), (f). This is because certain high k vector values, although present in the interference experiment, Figs. 14 (c) and (f), are not present in the measured dispersions (see Fig. 13 (b)) due to the limited size of the CCD detector in the spectrometer, thus their contribution is absent in the numerically reproduced interference image. Importantly, the most prominent features of the measured spatial coherence images can be numerically reproduced from the measured dispersion image (describing the dispersion of the modes) radiating through a double slit. Thus we can conclude that the complex pattern in the spatial coherence image

originates from the interference of the strongly coupled delocalized mode (i.e. the measured dispersion) at the double slit.

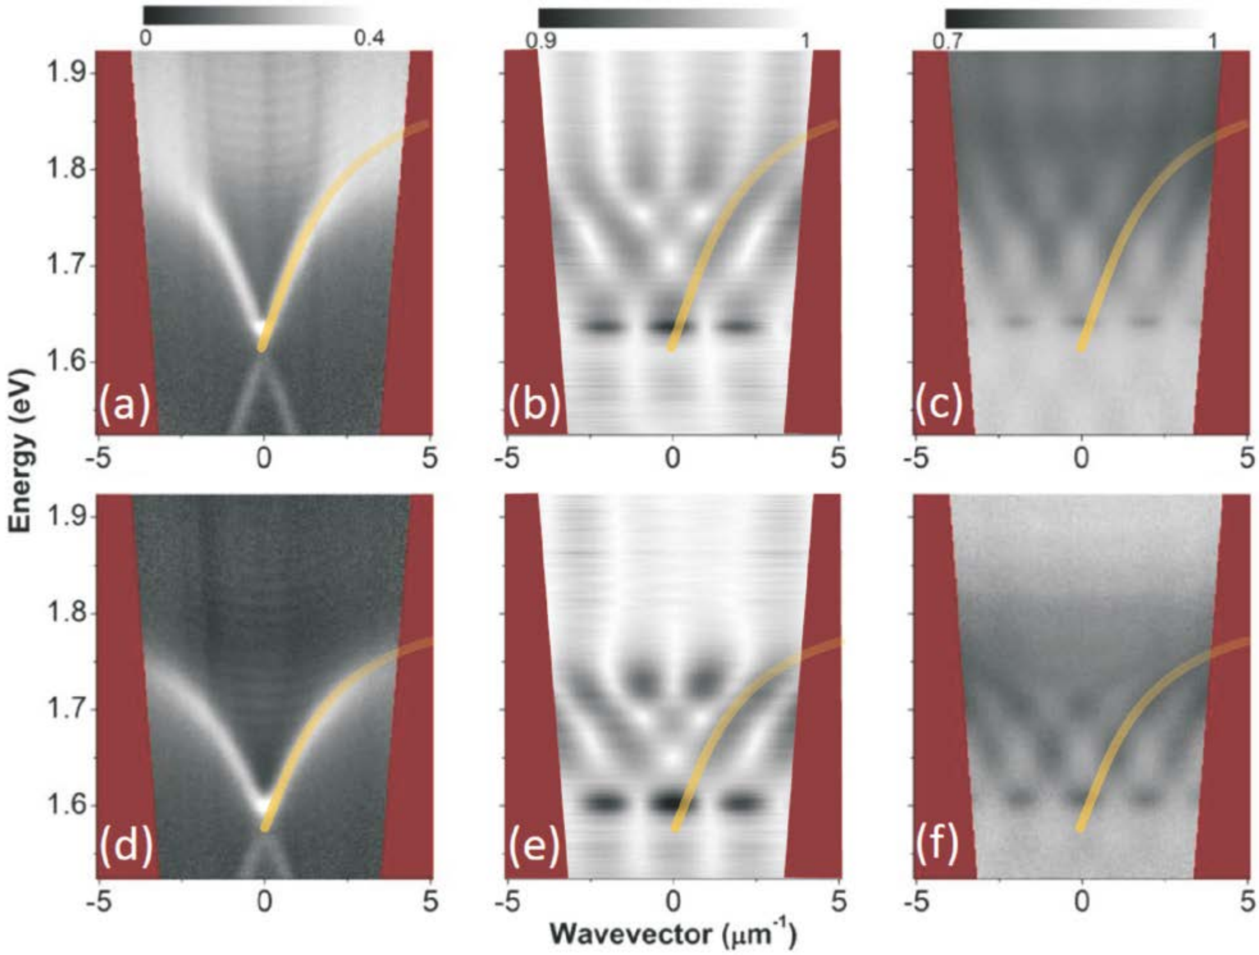


Fig. 14. (a) The measured dispersion, (b) the numerically generated spatial coherence image from the measured dispersion image, and (c) the experimentally obtained spatial coherence image for 400 mM DiD concentration. (d-f) The same for 800 mM DiD concentration. The yellow lines depict the extinction maxima of the dispersion curve. In the dispersions, we plot the extinction (1-T) as white color and for both spatial coherence images we plot the transmission T, as defined in the manuscript.

**References**


[1] V. M. Agranovich, M. Litinskaia, and D. G. Lidzey, Phys. Rev. B 67, 085311 (2003).

[2] A. Gonzalez-Tudela, P. A. Huidobro, L. Martin-Moreno, C. Tejedor and F. J. Garcia-Vidal, Phys. Rev. Lett. 110, 126801 (2013).

[3] R. A. L. Vallée, M. Van Der Auweraer, F. C. De Schryver, D. Beljonne, and M. Orrit, ChemPhysChem, 6, 81 (2005).
